# Supplementary material for: Unsupervised Corpus Aware Language Model Pre-training for Dense Passage Retrieval
Source: arXiv:2108.05540 source file (2021-08-12)
Supplement: Supplementary file 1 [file appendix.tex]

\section{Appendix}
\label{sec:appendix}
\subsection{Hyper Parameters Settings}
\paragraph{STS-b} The training follows hyper-parameter settings in \citet{reimers-gurevych-2019-sentence}, Adam optimizer, a learning rate of 2e-5 with linear schedule, and 4 epochs. For low data setup, we search best epoch number in \{4,8\} for BERT and apply those to all other pre-trained models.
\paragraph{Wikipedia Section Distinction} The training follows hyper-parameter settings in \citet{reimers-gurevych-2019-sentence}, Adam optimizer, a learning rate of 2e-5 with linear schedule and 1 epoch. For low data setup, we search best epoch number in \{1,4,8\} for BERT and apply those to all other pre-trained models.
\paragraph{Open QA} We follow hyperparameter settings in \citet{karpukhin-etal-2020-dense}, 128 batch size, 1 BM25 negative, in-batch negatives, 40 epochs, 1e-5 learning rate and linear schedule with warmup. Low data share the same setting as we found 40 epochs are enough for convergence.
\paragraph{Web Search} We train with Adam optimizer, learning rate of 5e-6 for 5 epochs with a total batch size of 64: 8 query $\times$ 8 passages. For low data setup, we search best epoch number in \{5, 10, 40\} for BERT and apply those to all other pre-trained models.
\subsection{Model Size}
In our experiments, Condenser during fine-tuning has the same number of parameters as BERT base, about 100 M. Adding the head during pre-training, there are roughly 120 M parameters. 

\subsection{ICT Model}
\label{app:ict}
Our ICT model comes from \citet{lee-etal-2019-latent}. It is trained with a batch size of 4096. ICT's effectiveness in low data setup was verified and thoroughly studied by \citet{chang2020pretraining}. \citet{chang2020pretraining} also introduces two other pre-training tasks Body First Selection and Wiki Link Prediction. They heavily depend on Wikipedia like structure and knowledge of the structure during pre-training and therefore does not apply in general situations. Meanwhile, adding them improves over ICT by only around 1\% and \citet{chang2020pretraining} has not released their model checkpoints. Therefore we chose to use the ICT checkpoint. 

Difficulties in reproducing these models come from the large batch requirement and the contrastive loss in ICT. Both \citet{lee-etal-2019-latent} and \citet{chang2020pretraining} find it critical to use large batch: \citet{lee-etal-2019-latent} uses a 4096 batch and \citet{chang2020pretraining} a 8192 batch. Both were trained with Google's cloud TPU. In comparison, our GPU can fit a batch of only 64. The contrastive loss uses the entire batch as the negative pool to learn the embedding space. Using gradient accumulation will reduce this pool size by several factors, leading to a bad pre-trained model. In comparison, our Condenser is based on instance-wise MLM loss and can naively use gradient accumulation.

We convert the original Tensorflow Checkpoint into Pytorch with huggingface conversion script. We don't use the linear projection layer that maps the 768 BERT embedding vector to 128 so that the embedding capacity is kept the same as retrievers in \citet{karpukhin-etal-2020-dense}.

\begin{table}[h]
\centering
\scalebox{0.9}{
\begin{tabular}{ l || c  | c }
\hline \hline
% \multicolumn{4}{c}{\textbf{Web Search}}\\
% \hline
 & MSMARCO Dev & DL2019 \\
Model & MRR@100 & NDCG@10 \\
\hline
% & Top-20 & Top-100 & Top-20 & Top-100\\
BM25 & 0.230 & 0.519 \\
DeepCT & 0.320 & 0.544  \\
\hline
BERT & 0.340 & 0.546     \\
ME-BERT & n.a. & 0.588 \\
ANCE &  0.382 & \textbf{0.615}  \\
\hline
Condenser & 0.375 & 0.569 \\
Condenser + HN & \textbf{0.404} & 0.597 \\
\hline \hline 
\end{tabular}
}
\caption{Full train setup on MSMARCO Document. Results not available are denoted `n.a.'}
\label{tab:marco-doc-full}
\vspace{-0.5cm}
\end{table}

\subsection{Document Retrieval}
\label{app:mdoc}
Recent works~\cite{xiong2021approximate,Luan2020SparseDA} explored retrieving long documents with the MSMARCO document ranking dataset~\cite{bajaj2018ms}. There are several issues with this data set. The training set is not directly constructed but synthesizing from the passage ranking data set label. \citet{xiong2021approximate} find that the judgment in its TREC DL2019 test set biased towards BM25 and other lexical retrieval systems than dense retrievers. Meanwhile, \citet{Luan2020SparseDA} find single vector representation has a capacity issue in encoding long documents. To prevent these confounding from affecting our discussion, we opted to defer the experiment to this appendix. Here we use two query sets, MSMARCO Document Dev and TREC DL2019. We report official metrics MRR@100 on Dev and NDCG@10 on DL2019. Results are recorded in \autoref{tab:marco-doc-full}. Condenser improves over BERT by a large margin and adding HN also boosts its performance. Condenser + HN performs the best on Dev. On the other hand, we see ANCE is the best on DL2019. We conjecture the reason is that use of BM25 negatives in many systems is not favorable towards DL2019 labels that favor lexical retrievers. The multi rounds of negative mining help ANCE get rid of the negative effect of BM25 negatives.

\subsection{Engineering Detail} 
We implement Condenser~(from BERT) in Pytorch~\cite{pytorch} based on the BERT implementation in huggingface transformers package~\cite{hf-transformers}. As our adjustments go only into the model architecture and the LM objective is kept unchanged, we only need to modify the modeling file and reuse the pre-training pipeline from huggingface.

\subsection{Link To Datasets}
\paragraph{Sentence Similarity} Cleaned up version can be found in the sentence transformer repo \url{https://github.com/UKPLab/sentence-transformers}.
\paragraph{Open QA} We use cleaned up open qa data from DPR \url{https://github.com/facebookresearch/DPR/}.
\paragraph{Web Search} MSMARCO data can found on its homepage \url{https://microsoft.github.io/msmarco/}.
